# Supplementary material for: SuperMann: a superlinearly convergent algorithm for finding fixed points of nonexpansive operators
Source: arXiv:1609.06955 source file (2018-03-14)
Supplement: Supplementary file 1 [file Latafat.tex]

\newcommand\imm[1]{\bar #1}%
\newcommand\E{\mathbb E}%
\begin{algorithm}
	\algcaption{Randomized GKM scheme}%
	\label{alg:RGKM}%
	\begin{algorithmic}[1]%
\newcommand\keyfont[1]{\textsc{#1}}%
\item[]%
	\begin{tabularx}{\linewidth}{@{}l@{~~}X@{}}
			\keyfont{Require}%
		&
			\(x^0\in\HH\),~
			\(\beta,\sigma\in(0,1)\).%
		\\
			\keyfont{Initialize}%
		&
			\(k=0\),~
			\(I=\set{1\ldots N}\).%
	\end{tabularx}
\STATE\label{step:RGKM:initial}%
	\keyfont{If } \(I=\emptyset\), \keyfont{ then stop}%
\STATE%
	Sample a random index \(j\in I\)%
\STATE%
	\keyfont{If } \(R_jx^k=0\), \keyfont{ then ~set } \(I\gets I\setminus\set j\) and go to step \ref{step:RGKM:initial}%
\STATE%
	Set \(I\gets\set{1\ldots N}\) and select an update direction \(d_j\in\HH_j\)%
\STATE\label{step:RGKM:LS}%
	Let \(\tau=\beta^m\), with \(m\in\N\) the smallest such that \(w=x^k+\tau\imm d_j\) satisfies
	\[
		\rho_j
	{}\coloneqq{}
		\innprod{R_jw}{x_j^k-T_jw}_{\HH_j}
	{}\geq{}
		\sigma\|R_jw\|_{\HH_j}\|R_jx^k\|_{\HH_j}
	\]
\STATE%
	Let \(x^{k+1}\in\HH\) be defined as
	\[	
		x^{k+1}_i
	{}\coloneqq{}
		\begin{cases}[c@{~~\text{if }}l]
			x^k_i & i\neq j\\
			x^k_j - \frac{\rho_j}{\|R_jw\|\mathrlap{_{\HH_j}}}~~R_jw & i=j.
		\end{cases}
	\]
\STATE%
	Set \(k\gets k+1\) and go to step \ref{step:RGKM:initial}.
\end{algorithmic}
\end{algorithm}

For simplicity, in this section we suppose that \(T\) (and consequently \(R\)) are FNE.
Suppose that \(\HH=\HH_1\oplus\cdots\oplus\HH_N\) for some Hilbert spaces \(\HH_i\) endowed with inner product \(\innprod{\cdot}{\cdot}_{\HH_i}\) and induced norm \(\|{}\cdot{}\|_{\HH_i}\), \(i=1\ldots N\).

For \(i=1\ldots N\) denote by \(\imm\HH_i\leq\HH\) the immersion of \(\HH_i\) into \(\HH\).
For \(x\in\HH\), denote \(x=(x_1,\cdots, x_N)\) with \(x_i\in\HH_i\), and let \(\imm x_i=\proj_{\imm H_i}x\); in particular, \(x=\imm x_1+\ldots+\imm x_N\) and \(\innprod{\imm x_i}{\imm x_j}=0\) for \(i\neq j\).

\(\func T\HH\HH\) will be decomposed accordingly as \(\func{T_i}{\HH}{\HH_i}\) (\ie such that \(T_ix\coloneqq(Tx)_i\)), and \(\imm T_i=\func{\proj_{\imm\HH_i}\circ T}{\HH}{\imm\HH_i}\); a similar notation applies to \(R\).
The following statement follows from \cite[Prop. 4.32]{bauschke2011convex}.
\begin{lem}
For all \(i=1\ldots N\) the operator \(\imm T_i\) is \avg[\nicefrac 23].
\end{lem}
For \(j=1\ldots N\) and \(w\in\HH\) we define
\begin{equation}
	C_w(j)
{}\coloneqq{}
	\set{z\in\HH}[
		\innprod{R_jw}{z_j-T_jw}_{\HH_j}\leq 0
	].
\end{equation}

\begin{prop}
The following hold:
\begin{enumerate}
\item\label{prop:CwZj}
	\(\displaystyle
		\fix\imm T_j
	{}={}
		\bigcap_{w\in\HH}C_w(j)
	\);
%%%%
\item\label{prop:ZjfixT}
	\(\displaystyle
		\fix T
	{}={}
		\bigcap_{j=1}^N\fix\imm T_j
	\).
\end{enumerate}
\begin{proof}
\begin{proofitemize}
\item\ref{prop:CwZj}:
	the inclusion ``\(\subseteq\)'' is trivial.
	Let \(z\) be in the set in the right-hand side.
	In particular, \(z\in C_z(j)\) and therefore
	\(
		0
	{}\geq{}
		\innprod{R_jz}{z_j-T_jz}_{\HH_i}
	{}={}
		\|R_jz\|_{\HH_i}^2
	\).
	Necessarily, \(R_jz=0\), \ie \(z\in\fix\imm T_j\).
%%%%
\item\ref{prop:ZjfixT}:
	trivial.\qedhere
\end{proofitemize}
\end{proof}
\end{prop}

\begin{thm}
Let \(\sigma\in(0,1)\) and a point \(x\in\HH\) be fixed, and let an index \(j\) be randomly sampled in \(\set{1\ldots n}\) with uniform distribution.
Suppose \(w\in\HH\) satisfies
\(
	\rho_j
{}\coloneqq{}
	\innprod{R_jw}{x_j-T_jw}_{\HH_j}
{}\geq{}
	\sigma\|R_jw\|_{\HH_j}\|R_jx\|_{\HH_j}
\),
and let \(x^+\in\HH\) be defined as
\[
	x_i^+
{}\coloneqq{}
	\begin{cases}[c@{~~\text{if }}l]
		x_i & i\neq j\\
		x_j - \frac{\rho_j}{\|R_jw\|\mathrlap{_{\HH_j}}}~~R_jw & i=j.
	\end{cases}
\]
Then,
\begin{enumerate}
\item\label{prop:random:GenMannproj}
	\(x^+=\proj_{C_w(j)}x\);
%%%%
\item\label{prop:random:DriftedKMFejer_random}
	\(
		\|x^+-z\|^2
	{}\leq{}
		\|x-z\|^2
		{}-{}
		\sigma^2\|R_jx\|_{\HH_j}^2
	\)
	for all \(z\in\fix\imm T_j\);
%%%%
\item\label{prop:random:DriftedKMFejer}
	in particular,
	\(
		\E\left[\|x^+-z\|^2\right]
	{}\leq{}
		\|x-z\|^2
		{}-{}
		\tfrac{\sigma^2}{N}
		\|Rx\|^2
	\)
	for all \(z\in\fix T\).
\end{enumerate}
\begin{proof}
A similar reasoning as in \cref{lem:DriftedKM} shows \ref{prop:random:GenMannproj} and \ref{prop:random:DriftedKMFejer_random}.
In turn, \ref{prop:random:DriftedKMFejer} easily follows.
\end{proof}
\end{thm}

\begin{lem}[Linesearch]\label{prop:random:LS}
Let \(\sigma\in(0,1)\), an index \(j\in\set{1\ldots n}\), a point \(x\in\HH\) and a direction \(d_j\in\HH_j\) be fixed.
If \(x\notin\fix T\), then there exists \(\bar\tau>0\) such that, for all \(\tau\in[0,\bar\tau]\), the point \(w=x+\tau\imm d_j\) satisfies
\[
	\innprod{R_jz}{z_j-T_jz}_{\HH_j}
{}\geq{}
	\sigma\|R_jw\|_{\HH_j}\|R_jx\|_{\HH_j}.
\]
\begin{proof}
For \(\tau\to 0\), we have \(w\to x\) and the desired inequality becomes
\(
	\|R_jx\|_{\HH_j}^2
{}\geq{}
	\sigma
	\|R_jx\|_{\HH_j}^2
\).
\end{proof}
\end{lem}

\begin{thm}[Randomized GKM scheme]
Consider the iterates generated by \Cref{alg:RGKM}.
Either the algorithm terminates in a finite number of iterations, with \(x^k\in\fix T\), or the following hold:
\begin{enumerate}
\item\label{prop:RGKM:Fejer}
	the sequence \(\seq{x^k}\) is Fejér-monotone with respect to \(\fix T\);
\item\label{prop:RGKM:l2}
	\(Rx^k\to 0\) a.s., and \(\seq{\E\left[\|Rx^k\|^2\right]}\in\ell^2\);
\item\label{prop:RGKM:weak}
	\hl{cannot show that (in expect./a.s/in prob.)} \(x^k\rightharpoonup x^\star\) for some \(x^\star\in\fix T\).
\end{enumerate}
\begin{proof}
\cref{prop:random:LS} ensures that the stepsize \(\tau\) is found in a finite number of backtrackings at step \ref{step:RGKM:LS}; in particular, the algorithm is well-defined.
Moreover, the condition \(I=\emptyset\) corresponds to \(R_jx^k=0\) for all \(j\in\set{1\ldots N}\), \ie \(Rx^k=0\), proving the claim in the case the algorithm terminates in a finite number of iterations.

Suppose now this is not the case.
\begin{proofitemize}
\item\ref{prop:RGKM:Fejer}:
	follows from \cref{prop:random:DriftedKMFejer_random}.
%%%%
\item\ref{prop:RGKM:l2}:
	for \(i=1\ldots N\), let \(K_i=\set{k\in\N}[j_k=i]\); then, a.s. each \(K_i\) will contain infinite many indices.
	From \cite[Thm. 3.2]{combettes2015stochastic} we have that \(\imm R_{j_k}x^k\to 0\) a.s.; in particular,
	\(
		\seq{\imm R_{j_k}x^k}[k\in K_i]
	{}={}
		\seq{\imm R_ix^k}[k\in K_i]
	{}\to{}
		0
	\)
	for all \(i=1\ldots N\).
	\hl{(Make sure the next statement is correct)}
	Since \(x^{k+1}_i=x^k_i\) whenever \(k\notin K_i\), it follows that \(\seq{\imm x^k_i}\) is Fejér monotone with respect to \(\proj_{\imm\HH_i}\fix\imm T_i\), and that
	\(
		\imm R_ix^k_i
	{}\to{}
		0
	\)
	for all
	\(
		i\in 1\ldots N
	\).
	This condition ensures that \(\weak\seq{\imm x^k_i}\subseteq\fix\imm T_i\) for all \(i=1\ldots N\); in turn, from \cite[Thm. 5.5]{bauschke2011convex} it follows that \(\imm x^k_i\to x^\star(i)\) for some \(x^\star(i)\in\fix\imm T_i\).
	Therefore,
	\[
		\textstyle
		x^k
	{}={}
		\sum_{i=1}^n\imm x^k_i
	{}\rightharpoonup{}
		\sum_{i=1}^n\imm x^\star(i).
	\]

	\cref{prop:random:DriftedKMFejer} reads
	\[
		\E^k\left[\|x^{k+1}-z\|^2\right]
	{}\leq{}
		\|x^k-z\|^2
		{}-{}
		\tfrac{\sigma^2}{N}
		\|Rx^k\|^2
	\quad
		\text{for all \(z\in\fix T\),}
	\]
	where \(\E^k\) denotes the expectation conditional to the knowledge of samplings up to iteration \(k\) (inclusive).
	For any \(K\in\N\), by telescoping the unconditional expectation \(\E\) it follows that
	\[
		\|x^0-z\|^2
	{}\geq{}
		\E\left[
			\|x^0-z\|^2-\|x^{K+1}-z\|^2
		\right]
	{}\geq{}
		\frac{\sigma^2}{N}
		\sum_{k=0}^K \E\left[\|Rx^k\|^2\right]
	\quad
		\text{for all \(z\in\fix T\)}
	\]
	which proves that \(\seq{\|Rx^k\|}\in\ell^2\).
%%%%
\item\ref{prop:RGKM:weak}:
	due to Fejér monotonicity, the sequence \(\seq{x^k}\) is bounded and in particular has weak sequential cluster points.
	Fix \(x^\star\in\weak\seq{x^k}\), and let \(K\subseteq\N\) be such that \(\seq{x_k}[k\in K]\rightharpoonup x^\star\).
	Let \(j_k\) denote the index sampled at iteration \(k\).
	Since \(K\) is infinite, there exists \(j\in\set{1\ldots N}\) such that \(j_k=j\) for infinite many occurrences \(k\in K\).
	By possibly further extracting, we may suppose that \(j_k=j\) for all \(k\in K\).
	Now, by telescoping \cref{prop:random:DriftedKMFejer_random} we obtain
	\begin{equation}\label{eq:telescopeR_j}
		\|x^0-z\|^2
	{}\geq{}
		\sigma^2
		\sum_{k\in\N}\|R_{j_k}x^k\|_{\HH_{j_k}}
	{}\geq{}
		\sigma^2
		\sum_{k\in K}\|R_jx^k\|_{\HH_j}
	\quad
		\text{for all \(z\in\fix T\).}
	\end{equation}
	In particular, \(\seq{R_jx^k}[k\in K]\to 0\), and from \cite[Cor. 4.18]{bauschke2011convex} we deduce that \(x^\star\in\fix\imm T_j\).
	\hl{And now...?}
	\begin{itemize}
	\item
		We should be able to show that \(\weak\seq{x^k}\subseteq\fix T\) a.s., so that we may conclude invoking \cite[Prop. 2.3(iv)]{combettes2015stochastic} with \(\phi(t)=t^2\) and \(\vartheta_k\equiv\eta_k\equiv\chi_k\equiv 0\).
	%%%%
	\item
		Or maybe something can be done with \cite[Cor. 2.7(i)]{combettes2015stochastic}?
		For such, we should be able to show that the sequence
		\(
			\sqrt{
				\E^{k-1}\left[
					\|Rx^k-\imm R_{j_k}x^k\|^2
				\right]
			}
		\)
		is a.s. summable.
	\qedhere
	\end{itemize}
\end{proofitemize}
\end{proof}
\end{thm}
