# Supplementary material for: SuperMann: a superlinearly convergent algorithm for finding fixed points of nonexpansive operators
Source: arXiv:1609.06955 source file (2018-03-14)
Supplement: Supplementary file 2 [file Proofs_Broyden.tex]

\begin{lem}\label{lem:UpdateFNorm}
Suppose that \(\HH\) is finite dimensional, and let \(\seq{B_k}\) be defined as the relaxed Broyden's update \eqref{subeq:Broyden} with respect to some \(\seq{\vartheta_k}\subset[0,2]\), starting from some \(B_0\in\linop\).
Then, for any \(G\in\linop\) and \(k\in\N\) it holds that
{\mathloose%
\begin{align*}
	\|B_{k+1}-G\|_{\HS[]}
{}\leq{} &
	\|B_k-G\|_{\HS[]}
	{}-{}
	\frac{
		\vartheta_k(2-\vartheta_k)
	}{
		2\|B_k-G\|_{\HS[]}
	}
	\frac{
		\|
			(B_k-G)s_k
		\|^2
	}{
		\|s_k\|^2
	}
	{}+{}
	\vartheta_k
	\frac{\|y_k-Gs_k\|}{\|s_k\|}
\end{align*}}%
where the second term in the right-hand side is by convention null if \(B_k=G\).
\begin{proof}
Let \(E_k\coloneqq B_k-G\) and let \(\proj\) denote the projection operator with respect to the \(\HS[]\)-norm.
From \eqref{eq:BroydenProjection} we have
\begin{equation}\label{eq:LemBroyden1}
	E_{k+1}
{}={}
	\proj_{S_k,\vartheta_k}B_k
	{}-{}
	G
{}={}
	\left(
		\proj_{S_k,\vartheta_k}B_k
		{}-{}
		\proj_{S_k,\vartheta_k}G
	\right)
	{}-{}
	\vartheta_k(\id-\proj_{S_k})G
\end{equation}
Applying \eqref{eq:ProjClambdaFNE} to the first term between brackets we obtain
\begin{align*}
	{\left\|
		\proj_{S_k,\vartheta_k}B_k
		{}-{}
		\proj_{S_k,\vartheta_k}G
	\right\|}_{\HS[]}^2
{}\leq{} &
	{\left\|
		E_k
	\right\|}_{\HS[]}^2
	{}-{}
	\vartheta_k(2-\vartheta_k)
	{\left\|
		(\id-\proj_{S_k})B_k
		{}-{}
		(\id-\proj_{S_k})G
	\right\|}_{\HS[]}^2
\\
{}\overrel{\eqref{eq:StandardBroyden}}{} &
	{\left\|
		E_k
	\right\|}_{\HS[]}^2
	{}-{}
	\vartheta_k(2-\vartheta_k)
	\frac{
		{\left\|
			E_ks_k
			{}\otimes{}
			s_k
		\right\|}_{\HS[]}^2
	}{
		\|s_k\|^4
	}
\\
{}\overrel{\eqref{eq:Rank1Norm}}{} &
	{\left\|
		E_k
	\right\|}_{\HS[]}^2
	{}-{}
	\vartheta_k(2-\vartheta_k)
	\frac{
		\|E_ks_k\|^2
	}{
		\|s_k\|^2
	}
\end{align*}
Using the inequality
\(
	\sqrt{\alpha^2-\beta^2}
{}\leq{}
	\alpha - \nicefrac{\beta^2}{2\alpha}
\)
which holds for any \(\alpha,\beta\) satisfying \(0\neq\alpha\geq|\beta|\geq0\), we then obtain
\begin{equation}\label{eq:LemBroyden2}
	\left\|
		\proj_{S_k,\vartheta_k}B_k
		{}-{}
		\proj_{S_k,\vartheta_k}G
	\right\|_{\HS[]}
{}\leq{}
	\|E_k\|_{\HS[]}
	{}-{}
	\frac{
		\vartheta_k(2-\vartheta_k)
	}{
		2\|E_k\|_{\HS[]}
	}
	\frac{
		\|E_ks_k\|^2
	}{
		\|s_k\|^2
	}
\end{equation}
Moreover,
\begin{equation}\label{eq:LemBroyden3}
	{\left\|
		(\id-\proj_{S_k})G
	\right\|}_{\HS[]}
{}\overrel{\eqref{eq:StandardBroyden}}{}
	\left\|
		\tfrac{y_k-Gs_k}{\|s_k\|^2}
		{}\otimes{}
		s_k
	\right\|_{\HS[]}
{}\overrel{\eqref{eq:Rank1Norm}}{}
	\frac{\|y_k-Gs_k\|}{\|s_k\|}.
\end{equation}
The triangular inequality on \eqref{eq:LemBroyden1} combined with \eqref{eq:LemBroyden2} and \eqref{eq:LemBroyden3} proves the claimed result.
\end{proof}
\end{lem}

\begin{appendixproof}{thm:SuperMannBroyden}
The specific modified Broyden's update ensures that all \(B_k\) are invertible; moreover, letting \(\gamma\) be a modulus of subregularity for \(R\) at \(x_\star\) we have
\begin{align*}
	\|w_k-x_\star\|
{}={} &
	\|
		x_k-x_\star
	{}+{}
		\tau_kB_k^{-1}Rx_k
	\|
{}\leq{}
	\|x_k-x_\star\|
	{}+{}
	\|B_k^{-1}\|
	\|Rx_k\|
\\
	\text{\footnotesize\cref{lem:AvgProp:KMResDecrease}}
	~
{}\leq{} &
	\|x_k-x_\star\|
	{}+{}
	\|B_k^{-1}\|
	\|Rx_k\|.
\end{align*}
From \cref{thm:SuperMann:Linear} we know that \(\seq{\|Rx_k\|}\) and \(\seq{\|x_k-x_\star\|}\) are linearly convergent, hence summable, and since \(\seq{B_k^{-1}}\) is bounded so is \(\|w_k-x_\star\|\).
We may use \cref{rem:Broydenw} to apply \cref{thm:BroydenDM}, and since \(d_k=-B_k^{-1}Rx_k\) and \(s_k=-\tau_kd_k\) we have
\[
	\lim_{k\to\infty}{
		\frac{
			\|Rx_k+G_\star d_k\|
		}{
			\|d_k\|
		}
	}
{}={}
	\lim_{k\to\infty}{
		\frac{
			\|(B_k-G_\star)d_k\|
		}{
			\|d_k\|
		}
	}
{}={}
	\lim_{k\to\infty}{
		\frac{
			\|(B_k-G_\star)s_k\|
		}{
			\|s_k\|
		}
	}
~{}\overrel{\eqref{eq:BroydenDM}}{}~
	0.
\]
Therefore, \eqref{eq:DM} holds and \cref{thm:Local} applies.

It follows that there exists a sequence \(\seq{\delta_k}\subset[0,+\infty)\) such that \(\delta_k\to 0\) and
\(
	\|Rx_{k+1}\|\leq\delta_k\|Rx_k\|
\).
Then, proceding as in \eqref{eq:xRlinear} we obtain
\(
	\|x_k-x_\star\|
{}\leq{}
	\hat\delta_k
\),
where
\(
	\hat\delta_k
{}\coloneqq{}
	\delta_0\delta_1\cdot\delta_{k-1}\sum_{j\in\N}\|Rx_j\|,
\)
the last sum being finite.
Since \(\nicefrac{\hat\delta_{k+1}}{\hat\delta_k}=\delta_k\to 0\), it follows that \(\seq{x_k}\) is \(R\)-superlinearly convergent;
because of \eqref{eq:distR}, so is \(\seq{\dist(x_k,\fix T)}\).
\end{appendixproof}
