# Supplementary material for: SuperMann: a superlinearly convergent algorithm for finding fixed points of nonexpansive operators
Source: arXiv:1609.06955 source file (2018-03-14)
Supplement: Supplementary file 3 [file Proofs_GenMann.tex]

\begin{appendixproof}{thm:GKM}
\begin{proofitemize}
	\item\ref{thm:GKM:Fejer}:
		follows from \cref{prop:DriftedKMFejer} and the lower bound on \(\rho_k\) at \cref{state:GKM:initial}.
	%%%%
	\item\ref{thm:GKM:Tau_k}:
		follows from \cref{thm:LS} together with the minimality of \(i_k\in\N\) in determining the stepsize \(\tau_k=\beta^{i_k}\); in particular, a feasible \(\tau_k\) is always obtained in finitely many backtrackings, proving the algorithm to be well defined.
	%%%%
	\item\ref{thm:GKM:ResStr} and \ref{thm:GKM:xWeak}:
		due to the bounds on \(\seq{\lambda_k}\), from \ref{thm:GKM:Fejer} it follows that
		\(
			\underline\sigma
		{}\coloneqq{}
			\sigma^2
			\lambda_k(\nicefrac1\alpha-\lambda_k)
		{}\geq{}
			\sigma^2\delta(1-\delta)
		{}>{}
			0
		\).
		In particular, the algorithm is a special instance of \cref{alg:General} with \(\sigma=\underline\sigma\) and \(c_0=c_1=q=0\).
		The sought proof then follows from \cref{{thm:General:ResStr},{thm:General:xWeak}}.
	%%%%
	%%%%
	%%%%
	\item\ref{thm:GKM:Linear}:
		suppose now that convergence is strong and that \(R\) is metrically subregular at the limit \(x_\star\) with modulus \(\gamma\) and radius \(\varepsilon\).
		Let \(\bar k\in\N\) be such that \(x_{\bar k}\in\ball{x_\star}{\varepsilon}\) for all \(k\geq\bar k\), and let \(z_k\coloneqq\proj_{\fix T}x_k\) (well-defined due to \cite[Cor. 4.15]{bauschke2011convex}).
		Let \(e_k\coloneqq\dist(x_k,\fix T)=\dist(x_k,\zer R)\); metric subregularity then reads
		\[
			\|x_k-z_k\|
		{}={}
			e_k
		{}\leq{}
			\gamma
			\|Rx_k\|
		\qquad
			\forall k\geq\bar k.
		\]
		From \ref{thm:GKM:Fejer} we obtain that for all \(k\geq\bar k\)
		\[
			e_{k+1}^2
		{}\leq{}
			\|x_{k+1}-z_k\|^2
		{}\leq{}
			\|x_k-z_k\|^2
			{}-{}
			\underline\sigma
			\|Rx_k\|^2
		{}\leq{}
			\rho^2
			e_k^2
		\]
		where
		\(
			\rho
		{}\coloneqq{}
			\sqrt{
				1-\frac{\underline\sigma}{\gamma^2}
			\,}
		\),
		proving \(Q\)-linear convergence rate of \(\seq{e_k}\).
		\(R\)-linear convergence of \(\seq{\|Rx_k\|}\) follows from the bound
		\(
			\|Rx_k\|
		{}\leq{}
			2\alpha\|x_k-z_k\|
		\)
		due to \(2\alpha\)-Lipschitz continuity of \(R\).
	%%%%
	%%%%
	%%%%
	\item\ref{thm:GKM:xLinear}:
		follows from the same reasoning as in \eqref{eq:xRlinear} using the bound
		\begin{align*}
			\|x_{k+1}-x_k\|
		{}={} &
			\frac{\lambda\rho_k}{\|Rw_k\|}
		{}\leq{}
			\lambda
			\left(
				\|Rw_k\|+2\alpha\tau_k\|d_k\|
			\right)
		\\
		{}\leq{} &
			\lambda
			\left(
				\|Rw_k-Rx_k\|+\|Rx_k\|+2\alpha D\|Rx_k\|
			\right)
		{}\leq{}
			\lambda(1+4\alpha D)
			\|Rx_k\|
		\qedhere
		\end{align*}
	%%%%
	%%%%
	%%%%
\end{proofitemize}
\end{appendixproof}
